# Supplementary material for: Intrinsic Harmonization for Illumination-Aware Compositing
Source: arXiv:2312.03698 source file (2023-12-07)
Supplement: Supplementary file 1 [file 10_supplementary.tex]

In this supplementary document, we provide
(1) training and inference details for the re-shading network.
(2) architectures, training details, and dataset generation process for our albedo harmonization network in Section~\ref{sec:supp:albedoharmonize},
(3) details of our user study in Section~\ref{sec:supp:userstudy}

\section{Shading Refinement}
Our re-shading network is trained at a resolution of $(384 x 384)$ with a batch size of $8$. For each batch, images are non-uniformly sampled from each of the 3 three datasets. We bias the sampling towards the multi-illumination dataset as the off-the-shelf intrinsic decomposition method is trained on this data and therefore generates reliable shading and albedo estimates. This means less shading information is left in the albedo and the re-shading network learns to generate novel outputs rather than recovering the source illumination conditions from cues in the albedo.

As described in Section 4.1 we use gradient-based optimization with constraints to determine optimal lighting model parameters during inference. During training, this process is too slow and we therefore remove the constraints and solve the optimization with least-squares. We perform least squares using the normals and shading of the foreground region rather than the background. This is possible since the original image is already harmonized, so we know this will give us reliable lighting parameters. Additionally, this allows the model to learn to rely on the Lambertian shading provided as input which results in a controllable lighting refinement network.

All images used in the figures and experiments are sent through our model at 1024-pixel resolution. We found that this was the largest resolution where the off-the-shelf estimators provide consistent results, and our model is able to generate enough details while still being globally coherent across the foreground region.

\begin{figure}
    \centering
    \includegraphics[width=\linewidth]{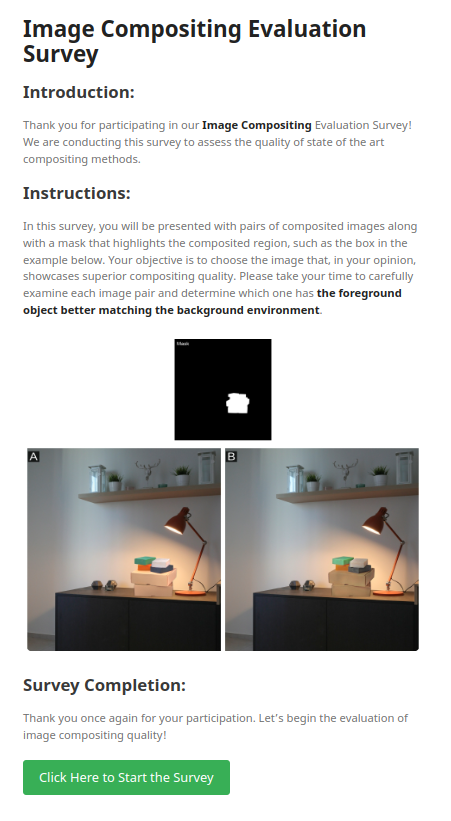}
    \caption{The instruction page of our user study. Image credit: Unsplash users Jean-Philippe Delberghe and Miguel Constantin Montes}
    \label{fig:userstudypage}
\end{figure}

\section{Albedo Harmonization}
\label{sec:supp:albedoharmonize}
\subsection{Training Data}

Our albedo harmonization network aims to regress a set of parameters for common image editing operations. To generate our training data we start with the estimated albedo from a natural image and edit a masked region such that it creates a mismatch with the rest of the image. 
To achieve that we exploit common image editing operations, such as exposure, saturation, and color changes. We select the edit operations and set parameter ranges as summarized in Table~\ref{tab:albedonet:params}.

We utilize MS-COCO~\cite{lin2014microsoft} and Davis~\cite{perazzi2016davis} dataset as they provide a segmentation mask for each of the objects present in the scene. During training, we randomly select one of the object masks in the scene. Next, we select a random number of edits (between 1-4), then an order for the edit operations, and values for each of the operations, sampled uniformly at random from the pre-specified ranges in Table~\ref{tab:albedonet:params} and apply the edit to the region specified by the mask. Some example training images are visualized in Figure~\ref{fig:supp:harmdataset}. 

\subsection{Network Architecture}

Given a naive composited albedo image and a region mask, our albedo harmonization network regresses multiple sets of parameters, one for each edit operation. We follow \citet{miangolehrealistic} and borrow their image editing network. They use their image editing network to regress image edits that increase or decrease the saliency of a specific region. 
We update the target ranges for the affine transforms of the estimation head of parameters in \citet{miangolehrealistic} to be $[0.1, 1]$ white balance, $[0, 2]$ saturation, $[0, 2]$ color curve values, and $[0.5, 2]$ exposure. 

We train the network using the ADAM optimizer (learning rate of $1e-5$) for 100 epochs with a batch size of 64. A random ordering of the 4 edit operations (out of 24 possible permutations) is sampled for each training batch and provided to the networks as input during training. We also select the permutation at random during inference.  

\begin{table}[t]
\caption{Edit operation definition and the parameter ranges used to generate naive composite training images for the albedo matching network.}
\resizebox{\linewidth}{!}
{
\begin{tabular}{l|lc}
             Operation          & Formulation &  Parameter range \\
             \hline             
             Exposure           &   $ I' =  p_{exp} \cdot I $                           & $[0.5, 2]$   \\
             Saturation         &   $ I'=RGB(h,p_{sat}\times s ,v) \quad$ h,s,v=HSV(I)         & $[0, 2]$    \\
             Color curve        &   As defined by ~\citet{hu2018exposure}                               & $[0.5, 2]$ \\
             White balance    &   $ I' =  p_{wb} \cdot I $ (channel-wise)             & $[0.3, 0.7]$    \\
\end{tabular}
}
\label{tab:albedonet:params}
\end{table}

\section{User Study Details}
\label{sec:supp:userstudy}
A screenshot of our user study instruction page is included in Figure~\ref{fig:userstudypage}. We included the following instruction text in our user study, \textit{"In this survey, you will be presented with pairs of composited images along with a mask that highlights the composited region, such as the box in the example below. Your objective is to choose the image that, in your opinion, showcases superior compositing quality. Please take your time to carefully examine each image pair and determine \textbf{which one has the foreground object better matching the background environment.}"}
